# Supplementary material for: RTL2M$\mu$PATH: Multi-$\mu$PATH Synthesis with Applications to Hardware Security Verification
Source: arXiv:2409.19478 source file (2024-09-28)
Supplement: Supplementary file 1 [file 13-appendix.tex]

\yao{TODO: a bibilography for the appendix}
\section{Supplemental Appendix}
%Supplemental Material}
\label{sec:supplemental}

\subsection{More Leakage Function Examples}
\label{sec:more_f_leak}
% \caroline{DONE}
Fig.~\ref{fig:leakage_func_examples_more} provides more leakage function examples, primarily for advanced processor optimizations surveyed in recent work~\cite{pandora:isca:21}. 

%\vspace{-20pt}
\begin{figure}[t]
    \begin{tcolorbox}[left=0pt,right=0pt,top=2pt,bottom=2pt]
    %\begin{framed}
    \footnotesize
    %~\cite{balakrishnan2003exploiting}
      \textcolor{ForestGreen}{{\RaggedLeft// \textbf{Register-file 0/1 compression}: \inst{ADD} in \inst{rename} stalls if no valid physical register or moves to \inst{issue} if available physical register.}}\\
      % free\_pool[idx] indicates if PRF[idx] is available for rename. ADD can substituted with any register-writing instruction. 
      %Any register-writing instruction can be a transmitter, but for illustration simplicity, we choose ADD as example
      %}}\\
     %\hline \\[-8pt]
     \noindent\hlt{$\mathsf{dst\;ADD\_rename(AND^S\;i1)}$}$\;\mathsf{:}$ \newline
     %\indent$\;\;\mathsf{path\_id = (\vee_i\;free\_pool[i] == 1)}$\\
     \indent$\;\;\mathsf{\textcolor{blue}{return}\;ite(((free\_pool[i1.PRF\_idx] == ite((}$\hlt{$\mathsf{i1.\itarg{arg0}}$}$\mathsf{ + }$\hlt{$\mathsf{i1.\itarg{arg1}}$}$\mathsf{)}$\\[2pt]
     \indent$\;\;\;\;\mathsf{\le 1, 1, 0))\wedge\;\vee_{idx}\;free\_pool[idx] == 1), }$\hlt{$\mathsf{\{issue\}, \{rename\}}$}$\mathsf{)}$
     %   \end{tabular}
     %   } 
       \\[5pt]
%       ~\cite{silentstore,lepak2000value}
       \noindent\textcolor{ForestGreen}{{\RaggedLeft// \textbf{Silent-store:} %\inst{rdata} is returned by \inst{ST}'s earlier \inst{SS\hbox{-}load} micro-op. 
     \inst{ST} in \inst{SQCHit} completes silently on a match of \inst{rdata} returned by \inst{ST}'s earlier \inst{SS\hbox{-}load} micro-op. }}\\
     % at SQCacheHit cycle, ST is reading value in the cache
 %{
 %      % \renewcommand{\arraystretch}{1.3}
 %    \setlength{\arrayrulewidth}{1pt}
 %     \begin{tabular}[t]{
 %       @{}>{\raggedright\arraybackslash} m{0.95\linewidth}
 %       }
     %\noindent\textcolor{ForestGreen}{\RaggedLeft// Precondition}\newline
 %    $\mathsf{Mem[}$\hlt{$\mathsf{i1.\itarg{addr}}$}$\mathsf{] ==\; }$\hlt{$\mathsf{i1.\itarg{data}}$}$\mathsf{\;\;cache[}$\hlt{$\mathsf{i0.\iparg{addr}}$}$\mathsf{] == Mem[}$\hlt{$\mathsf{i1.\itarg{addr}}$}$\mathsf{]}$$\mathsf{\;\;\;}$\\[2pt]
 %     \hline \\[-8pt]
     \noindent\hlt{$\mathsf{dst\;ST\_SQCHit(ST^N\;i0, ST^S\;i1)}$}$\mathsf{\;:}$ \newline
     \indent$\;\;\mathsf{SS\_ld = (Mem[}$\hlt{$\mathsf{i1.\itarg{addr}}$}$\mathsf{] ==\; }$\hlt{$\mathsf{i1.\itarg{data}}$}\newline
     \indent$\;\;\;\mathsf{\;\wedge\;rdata == }$$\mathsf{\;\;cache[}$\hlt{$\mathsf{i0.\iparg{addr}}$}$\mathsf{])}$ \newline 
 %    \hlt{$\mathsf{i0.\iparg{addr}}$}$\mathsf{\;==\; }$\hlt{$\mathsf{i1.\itarg{addr}}$}$\mathsf{\;\wedge \;}$\hlt{$\mathsf{i0.\iparg{data}}$}$\mathsf{\;== cache[}$\hlt{$\mathsf{i0.\iparg{addr}}$}$\mathsf{]}$\newline
     \indent$\;\;\mathsf{path\_id = (}$\hlt{$\mathsf{i0.\iparg{addr}}$}$\mathsf{\;==\; }$\hlt{$\mathsf{i1.\itarg{addr}}$}$\mathsf{\;\wedge \;}$\hlt{$\mathsf{i0.\iparg{data}}$}$\mathsf{\;== rdata)}$\newline
     \indent$\;\;\mathsf{\textcolor{blue}{return}\;ite((path\_id == 1), }$\hlt{$\mathsf{\{SQComp\}, \{reqWCache\}}$}$\mathsf{)}$ 
     \\ [5pt]
%     ~\cite{sodani1997dynamic}
       \noindent\textcolor{ForestGreen}{{\RaggedLeft// \textbf{Dynamic inst. reuse}: \inst{FP} in \inst{issue} computes (\inst{FPU}) or not depending on a single-entry reuse table that tracks prior \inst{FP} results.}}\\
    %{
    %    \renewcommand{\arraystretch}{1.3}
    % \setlength{\arrayrulewidth}{1pt}
    %  \begin{tabular}[t]{
    %    @{}>{\raggedright\arraybackslash} m{0.95\linewidth}
    %    }
     %\noindent\textcolor{ForestGreen}{\RaggedLeft// Precondition}\newline
 % \\[2pt]
  %   \hline
         \noindent\hlt{$\mathsf{dst\;FP\_issue(FP^N\;i0, FP^S\;i1)}$}$\;\mathsf{:}$\newline
         \indent$\;\;\mathsf{path\_id = (}$$\mathsf{reuse\_buffer == \{}$\hlt{$\mathsf{i1.\itarg{res}}$}$\mathsf{,}$\hlt{$\mathsf{i1.\itarg{arg0}}$}$\mathsf{,}$\hlt{$\mathsf{i1.\itarg{arg1}}$}$\mathsf{,i1.op\}\;\wedge}$ \newline 
         \indent$\;\;\;\;\mathsf{\{}$\hlt{$\mathsf{i0.\iparg{arg0},i0.\iparg{arg1}}$}$\mathsf{,i0.op\}== reuse\_buffer.\{arg0,arg1,op\})}$ \newline
     %\indent$\;\;\;\;\mathsf{}$\hlt{$\mathsf{i0.\iparg{arg1}}$}$\mathsf{ == i1.reuse\_buffer.arg1\;\wedge i0.op == reuse\_buffer.op})$ \newline
     \indent$\;\;\mathsf{\textcolor{blue}{return}\;ite((path\_id == 1), }$\hlt{$\mathsf{\{ROBComp\}, \{FPUnit\}}$}$\mathsf{)}$ \\ [5pt]
    %    \end{tabular}
    %} 
       \textcolor{ForestGreen}{{\RaggedLeft// \textbf{CVA6 \inst{ST} (cache):} A \inst{ST}, on a hit in the 4-way set-assoc. no-write-alloc. cache, will progress to update one of two data banks.}}\\ 
    \noindent\hlt{$\mathsf{dst\;ST\_wBVd(ST^N\;i0, ST^D\;i1, ST^S\;i2, LD^S\;i3, LD^D\;i4)}$}$\mathsf{\;:}$ \newline %\textcolor{ForestGreen}{// Leakage function}\newline
        \indent$\;\;\mathsf{todoBE = (set(}$\hlt{$\mathsf{i0.\iparg{addr}}$}$\mathsf{) == set(}$\hlt{$\mathsf{i1.\itarg{addr}}$}$\mathsf{)\;\wedge}$ \newline
        \indent$\;\;\;\;\mathsf{tag(}$\hlt{$\mathsf{i0.\iparg{addr}}$}$\mathsf{) == tag(}$\hlt{$\mathsf{i1.\itarg{addr}}$}$\mathsf{))\;\vee}$ \newline
        \indent$\;\;\;\;\mathsf{(set(}$\hlt{$\mathsf{i0.\iparg{addr}}$}$\mathsf{) == set(}$\hlt{$\mathsf{i2.\itarg{addr}}$}$\mathsf{)\;\wedge\;}$ \newline
        \indent$\;\;\;\;\mathsf{tag(}$\hlt{$\mathsf{i0.\iparg{addr}}$}$\mathsf{) == tag(}$\hlt{$\mathsf{i2.\itarg{addr}}$}$\mathsf{)) \wedge |be }$ \newline
        %\exists (cacheTag[set(}$\hlt{$\mathsf{i1.\itarg{addr}}$}$\mathsf{)][way] == tag(}$\hlt{$\mathsf{i1.\itarg{addr}}$}$\mathsf{)\;\wedge}$\newline 
        \indent$\;\;\mathsf{hit = (cacheTag[set(}$\hlt{$\mathsf{i1.\itarg{addr}}$}$\mathsf{)][way] == tag(}$\hlt{$\mathsf{i1.\itarg{addr}}$}$\mathsf{)\;\wedge}$\newline 
        \indent$\;\;\;\;\mathsf{set(}$\hlt{$\mathsf{i0.\iparg{addr}}$}$\mathsf{) == set(}$\hlt{$\mathsf{i1.\itarg{addr}}$}$\mathsf{)\;\wedge\;tag(}$\hlt{$\mathsf{i0.\iparg{addr}}$}$\mathsf{) == tag(}$\hlt{$\mathsf{i1.\itarg{addr}}$}$\mathsf{))}$ \newline
        \indent$\;\;\mathsf{\textcolor{blue}{return}\;ite(hit \wedge todoBE, }$\hlt{$\mathsf{\{wRTg, wr\$[way/2]\}, \{wRTg\}}$}$\mathsf{)}$ 
    \end{tcolorbox}
%    
%       \end{subfigure}%
%
    \caption{Leakage functions for advanced processor optimizations~\cite{pandora:isca:21}, and the full version of \inst{ST\_wBVd} from Fig.~\ref{fig:leakage_func_examples} in the main paper. 
    %$\mathsf{I^N/I^D/I^S}$: intrinsic/dynamic/static transmitter.
    %PO: Program order. \inst{ite(c,t,f)}: returns $t$ if $c$ is true or $f$ otherwise. $\mathsf{msb}$: Most significant bit.
    % \chris{define all the terms: PO, ite, msb, etc.}\yao{fixed}
    % \chris{I'm not sure this figure is adding much/whether people will read it beyond the ADD\_ID example}
    }
    % \yao{added a forward reference to result that discuss the leakage functions}
%    \caption{(Abstract) leakage function for different instruction at differing phases as defined in a \tspec{} model w.r.t optimizations in pandoras;
%    $\mathsf{I_P/I_I/I^D/I^S}$ is transponder/intrinsic transmitter/dynamic transmitter/static transmitter respectively. 
%    }
    \label{fig:leakage_func_examples_more}
\end{figure}

\subsection{SystemVerilog Assertion Preliminaries}
\label{sec:sva}

%To exhaustively explore the space of possible execution behaviors for some IUV executing on a particular DUV, \tsynth{} makes extensive use of LTL properties~\cite{pnueli:ltl,manna:ltl-textbook} formulated as SystemVerilog Assertions (SVAs)~\cite{vijayaraghavan:sva}, a SystemVerilog~\cite{ieee1800} language construct. 
% \caroline{DONE}
This section serves as a brief primer on LTL formulae~\cite{pnueli:ltl,manna:ltl-textbook} and SystemVerilog Assertions (SVAs)~\cite{vijayaraghavan:sva}. 

LTL formulae may be used to describe properties about the future states of an execution trace or execution \textit{path}.
LTL formulae are built over a base set of propositional variables, which act as the \textit{atoms} of the logic, and are used to describe basic properties of states within an execution trace.
The logic also contains the logical truth and falsity constants, as well as the standard connectives of propositional logic: conjunction ($\wedge$), disjunction ($\vee$), negation ($\neg$), and implication ($\rightarrow$).
These formulae are augmented with \emph{temporal modalities} which relativize a formula against an abstract notion of time, permitting formulae to make reference to events occurring later in an execution trace.
The properties $\square\phi$ and $\diamond\phi$ assert that $\phi$ holds in \emph{every} and \emph{some} future state of the trace, respectively.

SVAs support specifying LTL properties over the execution traces that can be realized on a SystemVerilog RTL implementation.
One can evaluate SVAs, over an unbounded space of execution traces, using property verifiers based on model checking~\cite{clarke:model_checking, baier:principles_of_model_checking}.
Two main SVA constructs are relevant for understanding the properties which \tsynth{} instantiates and evaluates. 
First, \texttt{assert} properties direct a model checker to prove that a specified LTL formula holds for \textit{all} execution traces.
A failed \texttt{assert} property produces a \textit{counterexample}---an execution trace which violates the assertion. 
Second, \texttt{cover} properties direct a model checker to search for and report \textit{any} execution trace which satisfies a given LTL formula. A \textit{covered/reachable} \texttt{cover} property returns an execution trace satisfying the LTL formula.
A \texttt{cover} property may be \textit{unreachable} in the case that no execution traces satisfying the LTL formula exists. 
% Note the duality of \texttt{assert} and \texttt{cover} properties---an \texttt{assert} property involving formula $\phi$ can be viewed as a \texttt{cover} property with respect to $\lnot\phi$. 
Model checking \texttt{assert} and \texttt{cover} properties may also return an \textit{undetermined} result indicating that the property cannot be proved or refuted, owing to a timeout or other resource constraint, perhaps.
Finally, SVA \texttt{assume} statements may be used to constrain the space of executions considered by a model checker when evaluating \texttt{assert} or \texttt{cover} properties, limiting the execution paths considered by the model checker to those that satisfy the assumed property.

% \caroline{I moved this here to the appendix. It needs a reference from the main text and an editing pass.}\yao{Fixed, added reference in 4.3.3. }

\subsection{CVA6 block diagram}
\label{a:cva6_block}
\begin{figure}[t!]
    \centering
     \includegraphics[width=0.9\linewidth]{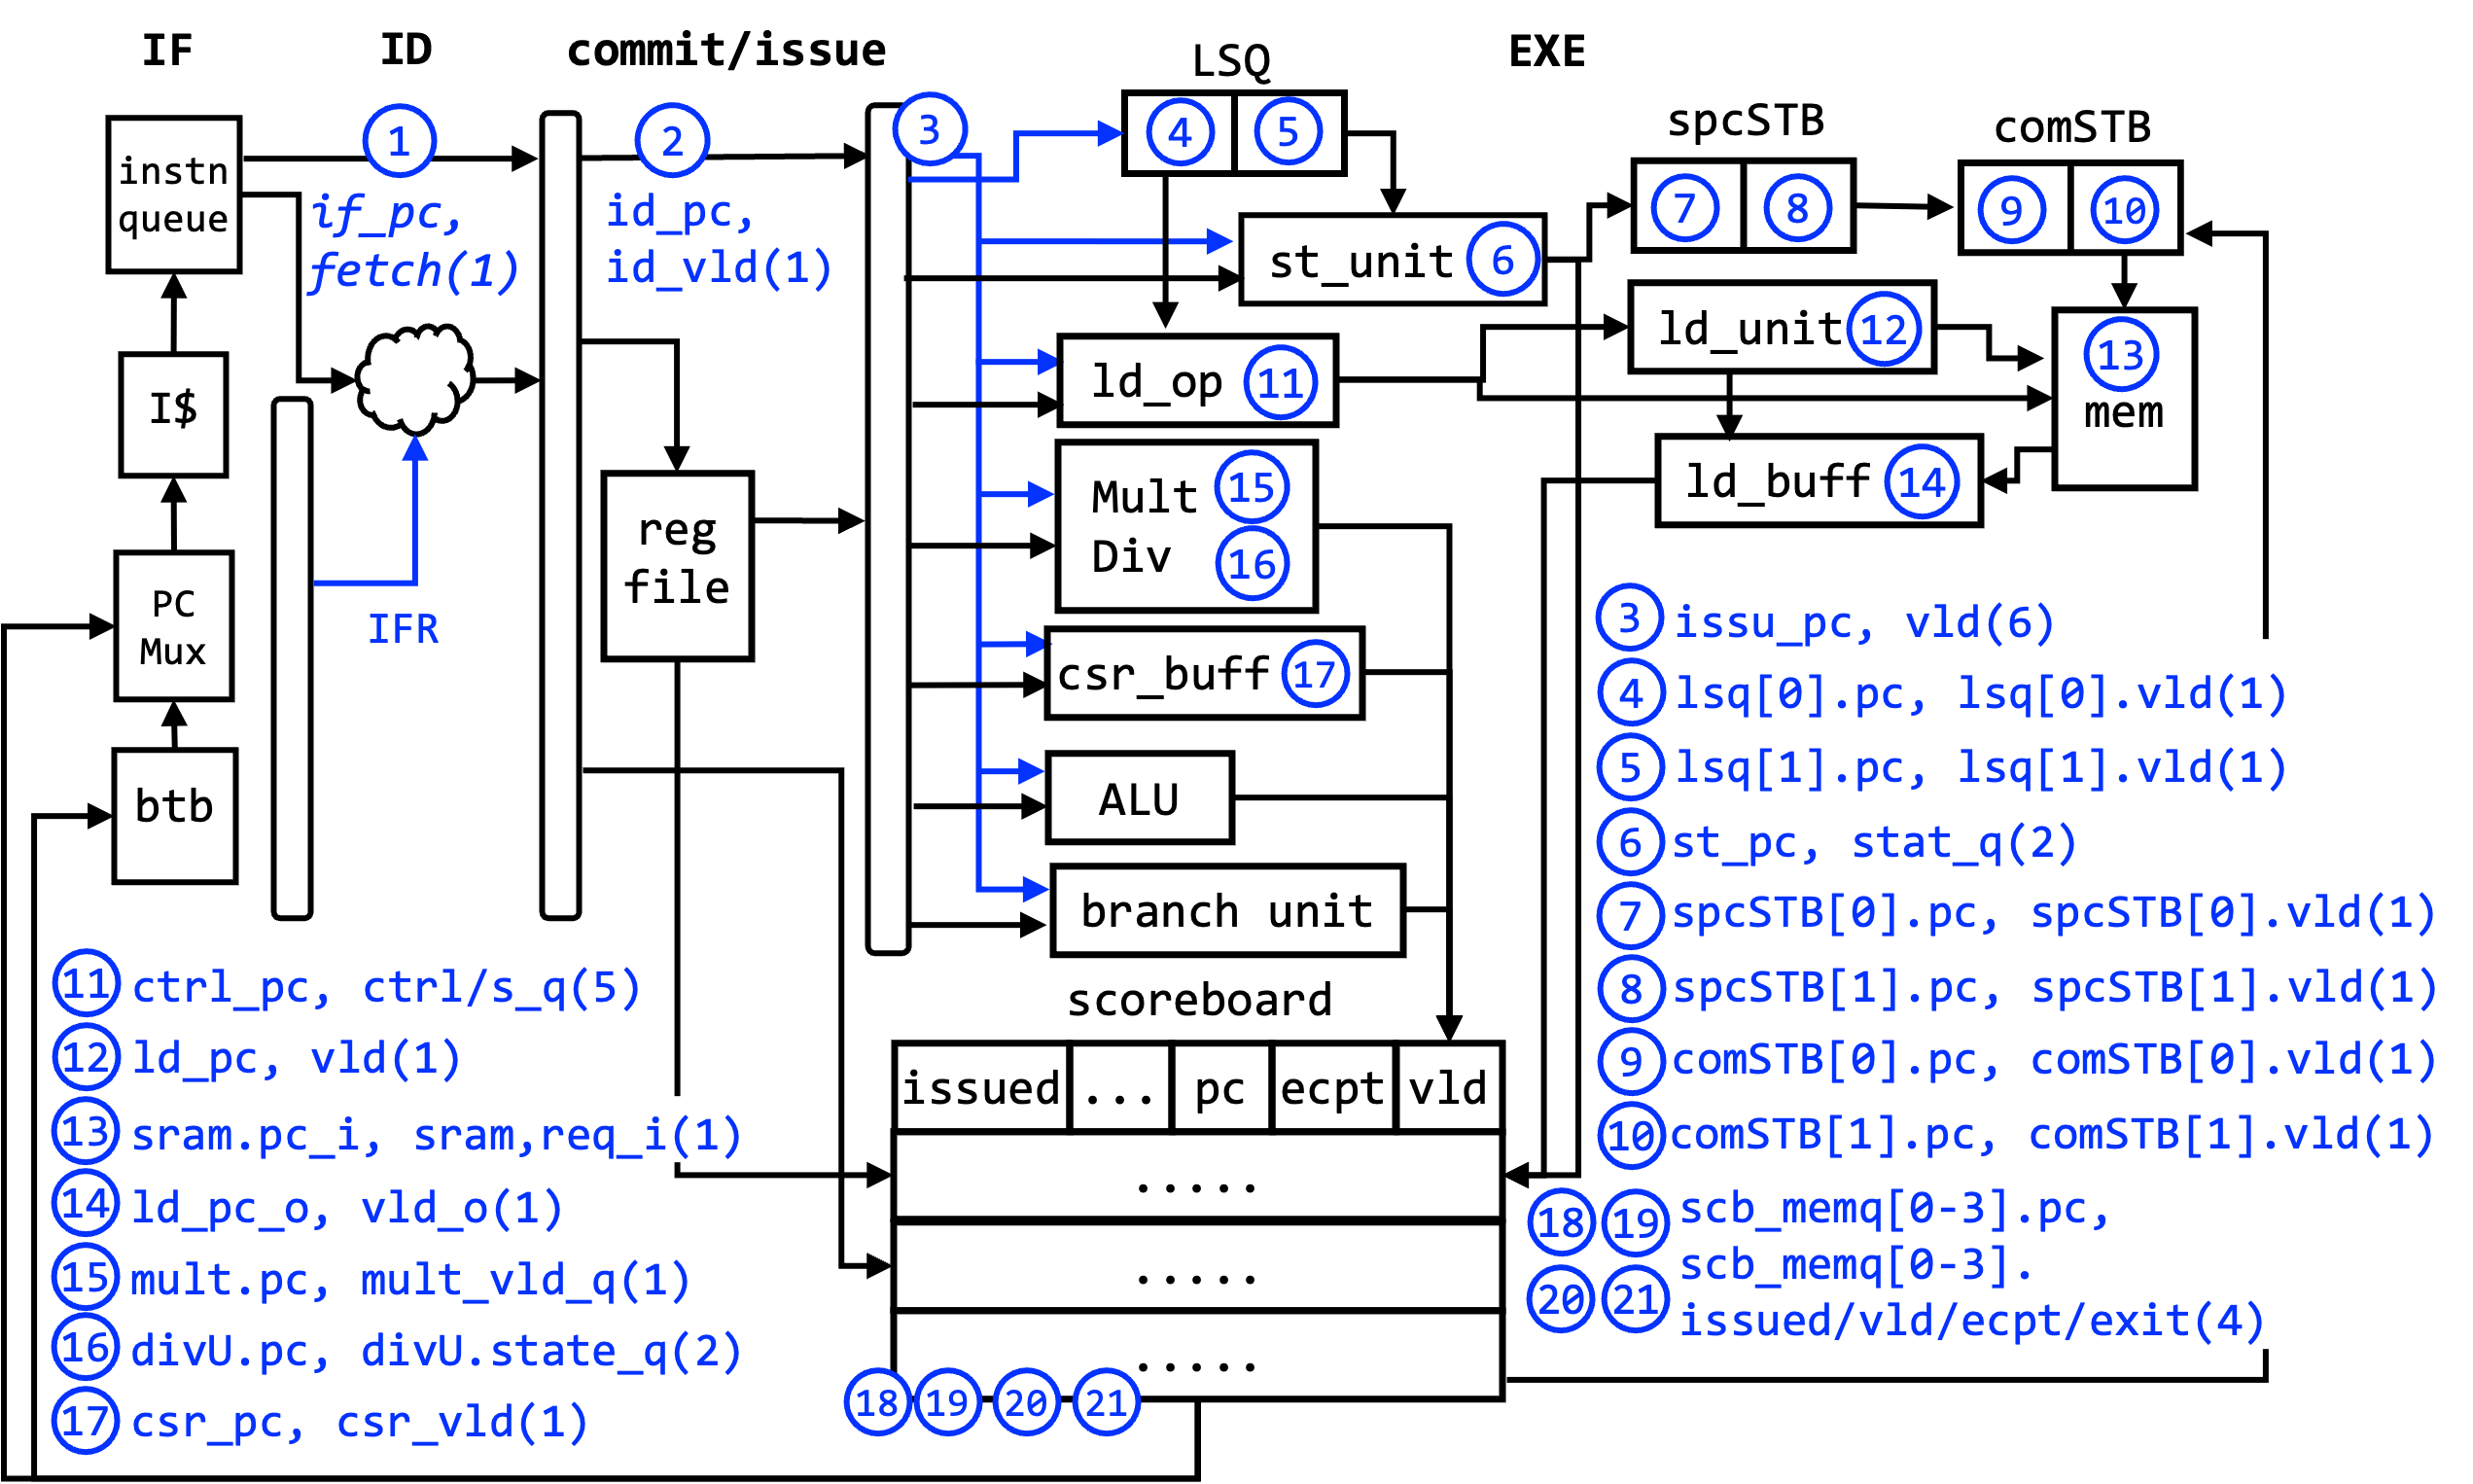}
     \caption{
     CVA6 block diagram. 1-21: $\langle \mathtt{IIR}, \mu \mathtt{FSM} \rangle$ pairs (\S\ref{sec:pls}). Bit-widths of \ufsm{} state variable(s) are given in parentheses.     %$\mathtt{PCR}$ and $\mu \mathtt{FSM}$ 
     % defined by state variable(s) with bit width in parentheses.
     %\inst{PCR_i} and $\mu FSM_i$ 
     %followed by \ufsm{} consisting of state variables 
     %CVA6 block diagram. 1-21:is a (PCR, \ufsm{}) tuple, where \ufsm{} are defined by state variables.
     %(PCR, \ufsm{}) tuples. 
     %A sample of synthesized \upaths{} on CVA6 with respect to data cache (for \inst{SW}) and core (for \inst{BEQ}, \inst{LW}, \inst{ADD}).
     % Row(F/L): an exec. phase (first/last consecutive visit). 
     }
     \label{fig:cva6_block_diag}

\end{figure}

Fig.~\ref{fig:cva6_block_diag} shows all (\inst{PCR}, \inst{\mu FSM})
pairs used to derive PLs for CVA6.
%For \inst{PCR}s that are added, they are added in parallel to the \inst{IIR}s (\S\ref{sec:tspec:pls}) present in the DUV. 
%An IDR is a register that holds information which uniquely identifies an \textit{in-flight} instruction. Examples include PCs, reorder buffer (ROB) or scoreboard (SCB) identifiers, or memory transaction identifiers; \inst{PCR}s are a special type of IDR.
%In the CVA6 block diagram in Fig.~\ref{fig:cva6_block_diag}, 
Blue signal names ending with ``\inst{.pc}'' denote \inst{PCR}s; there are 21 in total, 14 of which we add.

\subsection{CVA6 Bugs}
\label{sec:cva6_bug_report}
% \caroline{DONE} 
\tsynth{} helped us identify four bugs in the CVA6 Core. Three are new and fixes are accepted up-streamed: CVA6 enforces 1-byte-alignment for \inst{JALR} and 2-byte-alignment for \inst{JAL} when both require 4-byte alignment; conditional branches raise an exception on target misalignment regardless of branch outcome, but an exception is required only on taken branches. 
%Our report and fix are acknowledged by the maintainer.
One was already fixed: the issue counter width was declared incorrectly such that the scoreboard could leverage its full length.

\subsection{\caroline{Integrate into appendix}}
For virtually all realistic receivers, including $\mathnormal{R}_C$, Eq.~\ref{eq:non-interference} is trivially invalid for any program that features secret-dependent control-flow. For example, consider the code listing, 
%\inst{if~(sec)~\{seq~/*latency~L\hspace{-2pt}*\hspace{-2pt}/\}~else~
%\{seq'~/*latency~L'\hspace{-2pt}*\hspace{-2pt}/\}}
\inst{if(sec)\{seq~/\mathord{*}latency~L\mathord{*}/\}else\{seq'~/\mathord{*}latency~L'\mathord{*}/\}},
%\texttt{if (sec) \{seq /*latency L*/\} else \{seq' /*latency L'*/\}}
which features a secret-dependent conditional branch. Clearly, and independent of microarchitecture, 
there exists instruction sequences \inst{seq} and \inst{seq'} whose latencies \inst{L} and \inst{L'}, respectively, are different (\inst{L \neq L'}).
% there exists instruction sequences \inst{seq} and \inst{seq'} whose latencies are different (\inst{L \neq L'}).
Given our focus on \textit{hardware} side-channels, we assume that all programs $p$ feature the same sequence of instructions along all branches of secret-dependent control-flow instructions, i.e., \inst{seq = seq'} for the code listing above.
