# Supplementary material for: RTL2M$\mu$PATH: Multi-$\mu$PATH Synthesis with Applications to Hardware Security Verification
Source: arXiv:2409.19478 source file (2024-09-28)
Supplement: Supplementary file 2 [file 12-appendix-proof.tex]

\input{12-formal-synth-proof}
\clearpage
